# Supplementary material for: Revealing effective classifiers through network comparison
Source: arXiv:1403.2668 source file (2014-11-26)
Supplement: Supplementary file 1 [file Supplementary.pdf]

# SUPPLEMENTARY INFORMATION

## Revealing effective classifiers through network comparison

Lazaros K. Gallos and Nina H. Fefferman

## DATASETS

In our study we have used a number of datasets to build and analyze networks. A short description of these datasets and their sources is as follows:

a) *Animal affiliation networks.* We have compiled a set of 37 empirically determined 'social' networks in different species that can be found in the published literature. Association among individuals was defined by affiliative behavior, such as proximity, grooming interactions, etc. Our analysis included primate populations, herd mammals, marine mammals, fish, birds, insects, and reptiles. A detailed list of the species used, along with the references from where the networks were extracted, is shown in Table 1. The network sizes varied from 18 to 380 individuals. In some cases, we had more than one network for each species, depending on when the network was recorded. These cases are indicated in the nodes column of Table 1.

b) *Facebook in 100 Universities.* These networks are based on facebook friendship connections in 100 Colleges and Universities in USA on September 2005. The data have been made publically available [32] and have been analyzed in Ref. [33]. At the early stages of facebook, only students from specific Universities could create accounts in the site. The data that we use were recorded for the 100 first Universities that joined facebook, and contain friendships only within the same University, providing us with 100 independent networks. The networks are complete, in the sense that they contain all the existing nodes and all the connections at that time.

We isolated the largest clusters in each case. The University IDs that are used in Fig. 3a of the main text are shown in Table 2. In the same table we provide the values of the average degree and the student enrollment size of each University in 2005, which are used for the color coding of Fig. 3a. We downloaded the enrollment information from the datacenter of the *National Center for Education Statistics*: http://nces.ed.gov/ipeds/datacenter/ by creating a custom query for the 12-month full-time equivalent enrollment in the Academic year 2005-06.

c) *Arxiv co-authorship networks*. We downloaded the entire database of all papers submitted to arxiv.org from the beginning of the site in 1991 until December 31, 2012, using the Open Archive Initiative (oai2) protocol. The databases were parsed to identify unique authors and the authors of each paper. We used the site's classification of papers into 18 broad categories, and created one network for each category using all the papers in that field. The network nodes correspond to authors and a link suggests that these two nodes have co-authored at least one paper in this category. The 18 fields were the following, with the size of the largest cluster in the network shown in parentheses: Quantitative Biology (8618), Computer Science (30689), Quantitative Finance (1514), Math (52351), Statistics (6360), Physics / Astrophysics (71155), Physics / Condensed Mattter (85956), Physics / General Relativity (16189), Physics / High Energy Physics -Experiment (28806), Physics / High Energy Physics - Lattice (5130), Physics / High Energy Physics - Phenomenology (31991), Physics / High Energy Physics - Theory (21398), Physics / Mathematical Physics (10918), Physics / Nuclear Experiments (19933), Physics / Nuclear Theory (14121), Physics / Physics (61665), Physics / Quantum Physics (22926), Physics / Nonlinear Sciences (13). Due to the small size of the largest cluster in the Nonlinear Sciences field we did not consider this network in our study.

d) *Software networks*: We used networks of software from two sources: 1) The data for *junit*, *jmail*, *flamingo*, *jung*, *colt*, *org*, *java*, and *javax* were downloaded from http://lovro.lpt.fri.uni-lj.si/publications.jsp?show=ssc . The analysis of these data was done in [34]. The network is created by connections between the classes - nodes - in each software code. Two classes are considered to be connected through the following dependencies: inheritance, field, parameter and return. 2) We also used the software packages *Abiword*, *DigitalMaterial*, *Linux*, *Mysql*, *VTK*, and *XMMS* from Ref. [35], that were also constructed according to class collaboration.

e) *Internet* (evolving network). We downloaded the CAIDA Autonomous System graphs from January 2004 to November 2007 from the SNAP Stanford datasets in http://snap.stanford.edu/data/as-caida.html . The data are described and analyzed in Ref. [36]. Starting from January 2004, we used a total of 47 static snapshots which were roughly one month apart each. This allows us to monitor the evolution of the network over 3 years.

f) *Messages in an online social networking site* (evolving network). This dataset was downloaded from http://toreopsahl.com/datasets/#online_social_network and has been analyzed in [37]. It corresponds to online messages sent among students at the University of California, Irvive, through a "Facebook-like Social Network". The original form of the network was directed, so we projected it to an undirected form by ignoring the directionality of the links. Each message was time-stamped so we were able to follow the entire network evolution. Our starting point was when the first 500 links were created, and we sampled snapshots of the network with 1000, 2000, 4000, 8000, and 13838 links.

g) *Gnutella sharing*. We used the 9 snapshots of a peer-to-peer Gnutella network [38], where nodes represent hosts and links are the connections between these hosts. This is a directed network, so we used its undirected projection.

h) *Protein Interaction networks.* We used 9 protein interaction networks from BioGrid [39] for the following species: A. thaliana, C. elegans, D. melanogaster, H. sapiens, M. musculus, P. falciparum, R. norvegicus, S. cerevisiae, and S. pombe.

i) *Metabolic networks.* We used the 43 metabolic networks from Ref. [40].

j) *Road networks.* A node in this network represents an intersection and the links correspond to the roads that connect these intersections. The three state-wide networks we used were for California, Pennsylvania, and Texas [41].

k) *Thesauri networks.* We extracted the networks from 5 thesauri datasets, where nodes represent words and the links indicate that the two words are synonyms. These data were extracted from the LibreOffice Thesaurus and correspond to the following languages: English (UK), English (US), Spanish (AR), Spanish (ES), and Spanish (VE).

l) *Web networks.* The nodes in these networks represent webpages and the network links represent hyperlinks connecting these webpages [41]. We converted all links to undirected, and used the web network of Berkeley and Stanford, Google, Notre Dame, and Stanford. The datasets were downloaded from the Stanford SNAP database.

m) *Amazon co-purchase*. This network connects items that were frequently purchased together in amazon.com, as found by crawling software [42]. The networks were converted to undirected. We used four networks based on data collected on 2003 on these dates: March 2, March 12, May 5, June 1. The data were downloaded from the Stanford SNAP database.

## TABLE S1

| COMMON NAME | SCIENTIFIC NAME | POPULATION | CITATION | NOTES |
|---|---|---|---|---|
| 1. African Buffalo A | *Syncerus Cafer* | 39 | [1] | Network in May 2002 |
| 2. African Buffalo B | *Syncerus Cafer* | 64 | [1] | Aggregate Nov 01-Oct 03 |
| 3. African Elephant | *Loxodonta Africana* | 112 | [2] | |
| 4. Asian Elephant | *Elephas Maximus* | 105 | [2] | |
| 5. Bats | *Thyroptera Tricolor* | 55 | [3] | |
| 6. Brushtail Possums | *Trichosurus vulpecula* | 18 | [4] | |
| 7. Chimpanzees | *Pan troglodytes schweinfurthii* | 18 | [5] | |
| 8. Cichlids | *Neolamprologous pulcher* | 72 | [6] | |
| 9. Columbian Squirrel | *Spermophilus Columbianus* | 65 | [7] | |
| 10. Crows | *Corvus moneduloides* | 34 | [8] | |
| 11. Dolphins | *Tursiops truncates* | 62 | [9] | |
| 12. Fungus Beetle | *Bolitotherus cornutus* | 34 | [10] | |
| 13. Giraffes | *Giraffa camelopardalis reticulata* | 77 | [11,23] | |
| 14. Great Tits | *Parus Major* | 104 | [12] | |
| 15. Guiana Dolphins | *Sotalia Guianensis* | 49 | [13] | |
| 16. Guppies | *Poecilia reticulata* | 63 | [14] | |
| 17. Hyenas A | *Crocuta Crocuta* | 35 | [15] | Low-prey period 1999 |
| 18. Hyenas B | *Crocuta Crocuta* | 35 | [15] | High-prey period 1999 |
| 19. Hyenas C | *Crocuta Crocuta* | 35 | [15] | Low-prey period 2000 |
| 20. Lizards | *Egernia stokesii* | 37 | [16] | |
| 21.Longtailed Manakins | *Chiroxiphia linearis* | 156 | [17] | |
| 22.Marmot Meadows | *Marmota flaviventris* | 22 | [18] | |
| 23. Onagers | *Equus hemionus khur* | 28 | [19] | |
| 24. Orca | *Orcinus Orca* | 43 | [20] | |
| 25.Pigtailed Macaques | *Macaca nemestrina* | 48 | [21] | |
| 26. Pygmy Whales | *Feresa Attenuata* | 103 | [22] | |
| 27. Red Deer | *Cervus Elaphus* | 45 | [23] | |
| 28. Rhesus Macaques | *Macaca mulatta* | 23 | [24] | |
| 29. Sea Lions | *Zalophus wollebaeki* | 380 | [25] | |
| 30. Snubnosed Monkeys | *Rhinopithecus roxellana* | 58 | [26] | |
| 31. Sparrows | *Melospiza melodia* | 74 | [27] | |
| 32.Tasmanian Devil A | *Sarcophilus harrisii* | 27 | [28] | During mating season |
| 33.Tasmanian Devil B | *Sarcophilus harrisii* | 27 | [28] | After mating season |
| 34. Wild Baboons | *Papio anubis – Papio hamadryas* | 35 | [29] | |
| 35. Wild Meerkats | *Suricatta suricatta* | 24 | [30] | |
| 36.Wiretailed Manakins | *Pipra Filicauda* | 46 | [31] | |
| 37. Zebras | *Equus grevyi* | 23 | [19] | |

# TABLE S2

| ID | UNIVERSITY | ENROLLMENT | <k> |
|---|---|---|---|
| 1 | American | 10007 | 68.3 |
| 2 | Amherst | 1642 | 81.4 |
| 3 | Auburn | 23537 | 105.6 |
| 4 | Baylor | 14771 | 106.2 |
| 5 | Boston College | 14328 | 84.7 |
| 6 | Berkeley | 33901 | 74.4 |
| 7 | Bingham | 13588 | 72.6 |
| 8 | Bowdoin | 1666 | 75.0 |
| 9 | Brandeis | 5826 | 70.8 |
| 10 | Brown | 7904 | 89.6 |
| 11 | Boston University | 30202 | 64.8 |
| 12 | Bucknell | 3645 | 83.1 |
| 13 | CalPoly San Luis Obispo | 17618 | 62.5 |
| 14 | Caltech | 2178 | 43.7 |
| 15 | Carnegie | 9091 | 75.5 |
| 16 | Colgate | 2744 | 89.1 |
| 17 | Columbia | 21522 | 75.9 |
| 18 | Cornell | 19602 | 84.9 |
| 19 | Dartmouth | 6071 | 79.2 |
| 20 | Duke | 16151 | 102.5 |
| 21 | Emory | 14149 | 88.6 |
| 22 | FSU | 36615 | 74.6 |
| 23 | Georgetown | 16369 | 90.7 |
| 24 | GWU | 19630 | 77.2 |
| 25 | Hamilton | 1805 | 83.4 |
| 26 | Harvard | 26324 | 109.3 |
| 27 | Haverford | 1111 | 82.4 |
| 28 | Howard | 11276 | 101.2 |
| 29 | Indiana | 36366 | 87.8 |
| 30 | JMU | 16737 | 69.0 |
| 31 | Johns Hopkins | 17154 | 72.4 |
| 32 | Lehigh | 6102 | 78.2 |
| 33 | Maine | 9241 | 53.7 |
| 34 | Maryland | 31280 | 71.5 |
| 35 | Michigan Tech | 6125 | 43.7 |
| 36 | Michigan | 39240 | 78.2 |
| 37 | Middlebury | 2902 | 81.2 |
| 38 | Mississippi | 14681 | 116.2 |
| 39 | MIT | 10079 | 78.5 |
| 40 | MSU | 45166 | 69.1 |
| 41 | Marquette | 10344 | 84.2 |
| 42 | Northeastern | 19999 | 55.1 |
| 43 | Northwestern | 16976 | 92.7 |
| 44 | NotreDame | 10832 | 89.1 |
| 45 | NYU | 39783 | 66.2 |
| 46 | Oberlin | 2840 | 61.6 |
| 47 | Oklahoma | 23350 | 102.5 |
| 48 | Penn State | 41602 | 65.6 |
| 49 | Pepperdine | 7403 | 88.4 |
| 50 | Princeton | 7095 | 89.2 |
| 51 | Reed | 1201 | 39.1 |
| 52 | Rice | 5321 | 90.5 |
| 53 | Rochester | 11364 | 70.8 |
| 54 | Rutgers | 31563 | 63.9 |
| 55 | Santa Clara | 8075 | 84.8 |
| 56 | Simmons | 4184 | 43.7 |
| 57 | Smith | 3118 | 65.4 |
| 58 | Stanford | 14087 | 98.1 |
| 59 | Swarthmore | 1452 | 73.7 |
| 60 | Syracuse | 16955 | 79.8 |
| 61 | Temple | 32740 | 52.8 |
| 62 | Tennessee | 17045 | 90.8 |
| 63 | U. Texas Austin | 46135 | 77.3 |
| 64 | Texas A&M | 42566 | 87.5 |
| 65 | Trinity | 2116 | 85.7 |
| 66 | Tufts | 11100 | 74.9 |
| 67 | Tulane | 8191 | 73.4 |
| 68 | U. Calif. Davis | 29394 | 62.2 |
| 69 | U. Calif. Irvine | 25781 | 64.4 |
| 70 | U. Calif. Riverside | 16443 | 45.6 |
| 71 | UCF | 39139 | 57.4 |
| 72 | UChicago | 9840 | 63.4 |
| 73 | UCLA | 36864 | 73.1 |
| 74 | UConn | 20672 | 70.3 |
| 75 | U.Calif. Santa Barbara | 21938 | 64.7 |
| 76 | U. Calif. Santa Cruz | 15265 | 50.0 |
| 77 | U. Calif. San Diego | 26291 | 59.3 |
| 78 | Univ. Florida | 52396 | 83.5 |
| 79 | UGA | 32539 | 96.3 |
| 80 | U. Illinois | 43572 | 82.1 |
| 81 | U. Mass. Amherst | 22601 | 62.9 |
| 82 | UNC Chapel Hill | 25757 | 84.5 |
| 83 | UPenn | 26686 | 92.2 |
| 84 | USC Columbia | 24467 | 92.0 |
| 85 | USF | 37461 | 48.1 |
| 86 | U. San Fransisco | 8599 | 48.8 |
| 87 | U. Virginia | 22977 | 91.9 |
| 88 | Vanderbilt | 10260 | 106.1 |
| 89 | Vassar | 2451 | 77.7 |
| 90 | Vermont | 10426 | 52.2 |
| 91 | Villanova | 9559 | 81.2 |
| 92 | Virginia | 27840 | 65.5 |
| 93 | Wake | 6662 | 104.1 |
| 94 | Washington U. St Louis | 12197 | 95.1 |
| 95 | Wellesley | 2505 | 63.9 |
| 96 | Wesleyan | 3515 | 76.9 |
| 97 | William & Mary | 7638 | 82.3 |
| 98 | Williams College | 2076 | 81.1 |
| 99 | Wisconsin | 35337 | 70.2 |
| 100 | Yale | 11288 | 94.7 |

## REFERENCES FOR THE SUPPLEMENTARY INFORMATION SECTION

[1] P.C. Cross, J.O. Lloyd-Smith, J.A. Bowers, C.T. Hay, M. Hofmeyr, & W.M. Getz, *Annales Zoologici Fennici* 41, 879 (2004).

[2] S. de Silva & G. Wittemyer, *Int. J. Primatol.* 33, 1125 (2012).

[3] G. Chaverri, *Behav. Ecol. Sociobiol.* 64, 1619 (2010).

[4] L.A.L. Corner, D.U. Pfeiffer, & R.S. Morris, *Preventive Veterinary Medicine* 59, 147 (2003).

[5] C.M. Murray, *Int. J. Primatol.* 28, 853 (2007).

[6] R. Schürch, S. Rothenberger, & and D. Heg, *Phil. Trans. R. Soc. B* 365, 4089 (2010).

[7] T.G. Manno, *Animal Behaviour* 75, 1221 (2008).

[8] C. Rutz, Z.T. Burns, R. James, S.M.H. Ismar, J. Burt, B. Otis, J. Bowen, & J.J.H. St Clair, *Current Biology* 22, R669 (2012)

[9] D. Lusseau, K. Schneider, O.J. Boisseau, P. Haase, E. Slooten, S.M. Dawson, *Behav. Ecol. Sociobiol.* 54, 396 (2003).

[10] V.A. Formica, C.W. Wood, W.B. Larsen, R.E. Butterfield, M.E. Augat, H.Y. Hougen, & E.D. Brodie III, *J. Evol. Biol.* 25, 130 (2012).

[11] B. Shorrocks & D.P. Croft, *Afr. J. Ecol.* 47, 374 (2009).

[12] I. Psorakis, S.J. Roberts, I. Rezek, & B.C. Sheldon, *J. R. Soc. Interface* 9, 3055 (2012).

[13] M. Cantor, L.L. Wedekin, P.R. Guimarães, F.G. Daura-Jorge, M.R. Rossi-Santos, & P.C. Simões-Lopes, *Animal Behaviour* 84, 641 (2012).

[14] D.P. Croft, J. Krause, S.K. Darden, I.W. Ramnarine, J.J. Faria, & R. James, *Behav. Ecol. Sociobiol.* 63, 1495 (2009).

[15] K.E. Holekamp, J.E. Smith, C.C. Strelioff, R.C. Van Horn, & H.E. Watts, *Molecular Ecology* 21, 613 (2012).

[16] S.S. Godfrey, C.M. Bull, R. James, & K. Murray, *Behav. Ecol. Sociobiol.* 63, 1045 (2009).

[17] D.B. McDonald, *Proc. Natl. Acad. Sci USA* 104, 10910 (2007).

[18] D.T. Blumstein, T.W. Wey, & K. Tang, *Proc. R. Soc. B* 276, 3007 (2009).

[19] S.R. Sundaresan, I.R. Fischhoff, J. Dushoff, & D.I. Rubenstein, *Oecologia* 151, 140 (2007).

[20] P.R. Guimarães, Jr., M.A. de Menezes, R.W. Baird, D. Lusseau, P. Guimarães, & S.F. dos Reis, *Phys. Rev. E* 76, 042901 (2007).

[21] J.C. Flack, M. Girvan, F.B.M. de Waal, & D.C. Krakauer, *Nature* 439, 426 (2006).

[22] D.J. McSweeney, R.W. Baird, S.D. Mahaffy, D.L. Webster, & G.S. Schorr, *Marine Mammal Science* 25, 557 (2009).

[23] D.P. Croft, R. James, & J. Krause, *Exploring Animal Social Networks* (Princeton Univ. Press , 2008).

[24] C.M. Berman, K.L.R. Rasmussen, & S.J. Suomi, *Animal Behaviour*, 53, 405 (1997).

[25] J.B.W. Wolf & F. Trillmich, *Proc. Biol. Sci.* 275, 2063 (2008).

[26] P. Zhang, B. Li, X. Qi, A.J.J. MacIntosh, & K. Watanabe, *Int. J. Primatol.* 33, 1081 (2012).

[27] C.N. Templeton, V.A. Reed, S.E. Campbell, & M.D. Beecher, *Behavioral Ecology* 23, 141 (2012).

[28] R.K. Hamede, J. Bashford, H. McCallum, & M. Jones, *Ecology Letters* 12, 1147 (2009).

[29] K. Sugawara, *Primates* 20, 21 (1979).

[30] J.R. Madden, J.A. Drewe, G.P. Pearce, & T.H. Clutton-Brock, *Behav. Ecol. Sociobiol.* 64, 81 (2009).

[31] T.B. Ryder, D.B. McDonald, J.G. Blake, P.G. Parker, & B.A. Loiselle, *Proc. R. Soc. B* 275, 1367 (2008).

[32] http://people.maths.ox.ac.uk/~porterm/data/facebook100.zip

[33] A.L. Traud, P.J. Mucha, & M.A. Porter, *Physica A*, 391, 4165 (2012).

[34] L. Subelj & M. Bajec, *Physica A* 390, 2968 (2011).

[35] C.R. Myers, *Phys. Rev. E* 68, 046116 (2003).

[36] J. Leskovec, J. Kleinberg, & C. Faloutsos. ACM SIGKDD International Conference on Knowledge Discovery and Data Mining (KDD), (2005).

[37] T. Opsahl, & P. Panzarasa, *Social Networks* 31, 155 (2009).

[38] J. Leskovec, J. Kleinberg and C. Faloutsos. ACM Transactions on Knowledge Discovery from Data (ACM TKDD), 1(1) (2007).

[39] C. Stark, B. J. Breitkreutz, T. Reguly, L. Boucher, A. Breitkreutz, and M. Tyers, *Nucleic Acids Research* 34, D535 (2006).

[40] H. Jeong, B. Tombor, R. Albert, Z. N. Oltvai, and A.-L. Barabasi, *Nature* 407, 651 (2000).

[41] J. Leskovec, K. Lang, A. Dasgupta, M. Mahoney. *Internet Mathematics* 6, 29 (2009).

[42] J. Leskovec, L. Adamic and B. Adamic. ACM Transactions on the Web (ACM TWEB), 1(1), 2007.
